# Supplementary material for: Greedy Matroid Algorithm And Computational Persistent Homology
Source: arXiv:2308.01796 source file (2023-08-03)
Supplement: Supplementary file 1 [file 09appendix2.tex]

\newpage
\begin{table}[!htb]
\footnotesize
    \begin{tabular*}{0.5\columnwidth}{@{\extracolsep{\fill}}ccc}
    \hline
        index   & size & $H_1$ \\\hline
        0:1000  & 1000 & [[1, 0], [0, 1]] \\\hline
        0: 20   & 20   & [[1, 0], [0, 2]] \\
        20:40   & 20   & [[1, 0], [0, 1]]\\
        100:120 & 20   & [] \\
        140:160 & 20   & [] \\
        180:200 & 20   & [] \\
        200:220 & 20   & [[2, 0], [1, 1]] \\
        500:520 & 20   & [[1, 0], [0, 1]]\\
        600:620 & 20   & [] \\
        900:920 & 20   & [[1, 0], [0, 2]]\\
        980:1000& 20   & [] \\
    \end{tabular*}
    \label{tab:fig_8_20_pm}
    \begin{tabular*}{0.5\columnwidth}{@{\extracolsep{\fill}}ccc}
    \hline
        index   & size & $H_1$ \\\hline
        0:1000  & 1000 & [[1, 0], [0, 1]] \\\hline
        0: 50   & 50   &  [[0, 2], [2, 0]] \\
        50:100  & 50   &  [[1, 1], [0, 2]] \\
        100:150 & 50   &  [[1, 0], [0, 2]] \\
        150:200 & 50   &  [[0, 1], [2, 0]] \\
        200:250 & 50   &  [[2, 2], [2, 0]] \\
        500:550 & 50   &  [[2, 0], [0, 1]] \\
        750:800 & 50   &  [[2, 0], [0, 2]] \\
        850:900 & 50   &  [[0, 1], [2, 0]] \\
        900:950 & 50   &  [[0, 2], [2, 0]] \\
        950:1000& 50   &  [[1, 0], [0, 2]] \\
    \end{tabular*}
    \label{tab:fig_8_50_pm} 
   \linebreak
   \linebreak
    \begin{tabular*}{0.5\columnwidth}{@{\extracolsep{\fill}}ccc}
    \hline
        index   & size  & $H_1$ \\\hline
        0:1000  & 1000  & [[1, 0], [0, 1]] \\\hline
        0:100   & 100   & [[1, 1], [0, 2]] \\
        100:200 & 100   &  [[1, 0], [0, 2]] \\
        200:300 & 100   &  [[1, 1], [2, 0]]\\
        300:400 & 100   &  [[1, 0], [0, 1]] \\
        400:500 & 100   &  [[0, 1], [1, 0]] \\
        500:600 & 100   &  [[2, 0], [0, 1]] \\
        600:700 & 100   &  [[0, 1], [2, 0]] \\
        700:800 & 100   & [[0, 1], [2, 0]] \\
        800:900 & 100   & [[2, 0], [0, 2]] \\
        900:1000& 100   & [[0, 1], [1, 0]] \\
    \end{tabular*}
    \label{tab:fig_8_100_pm}
    \begin{tabular*}{0.5\columnwidth}{@{\extracolsep{\fill}}ccc}
    \hline
        index   & size  & $H_1$ \\\hline
        0:1000  & 1000  & [[1, 0], [0, 1]]\\\hline
        0:300   & 300   & [[0, 1], [2, 0]]\\
        300:600 & 300   &  [[0, 2], [1, 0]]\\
        600:900 & 300   &  [[0, 1], [2, 0]]\\
        200:500 & 300   &  [[1, 0], [0, 1]]\\
        500:800 & 300   &  [[2, 0], [0, 2]]\\
        700:1000& 300   &  [[2, 0], [0, 2]]\\
        400:700 & 300   &  [[0, 2], [1, 0]]\\
        50:350  & 300   & [[0, 1], [2, 2]]\\
        287:587 & 300   & [[2, 0], [0, 2]]\\
        659:959 & 300   & [[2, 0], [0, 1]]\\
    \end{tabular*}
    \label{tab:fig_8_300_pm}
\caption{Projection maps of Figure-$8$ of size $1000$. Sub-sample size is $300$. Samples are randomly sampled from the full point cloud.} \label{tab:fig_8_pm}   
\end{table}

\newpage
\begin{figure}
    \centering
    \includegraphics[width=0.49\linewidth]{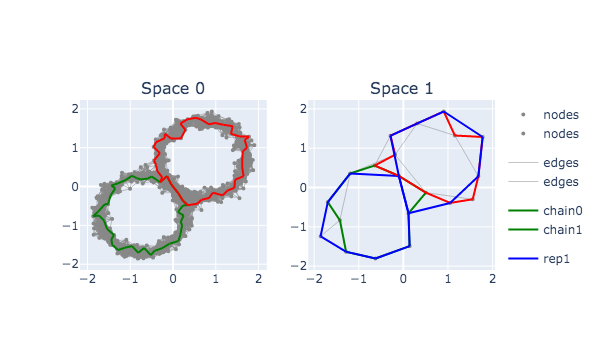}
    \includegraphics[width=0.49\linewidth]{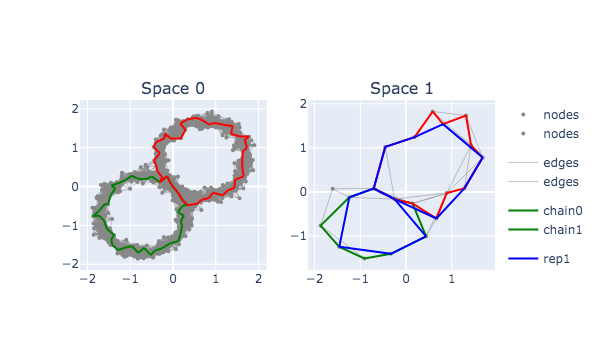}
    \includegraphics[width=0.49\linewidth]{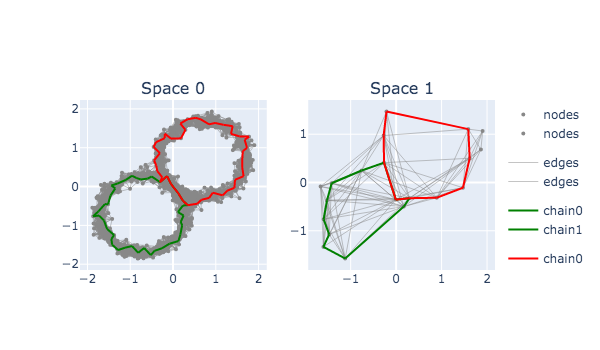}
    \includegraphics[width=0.49\linewidth]{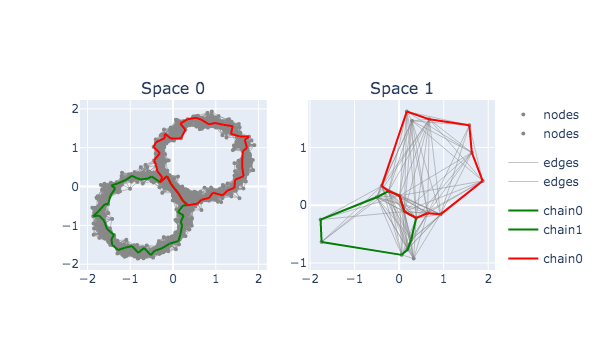}
    \includegraphics[width=0.49\linewidth]{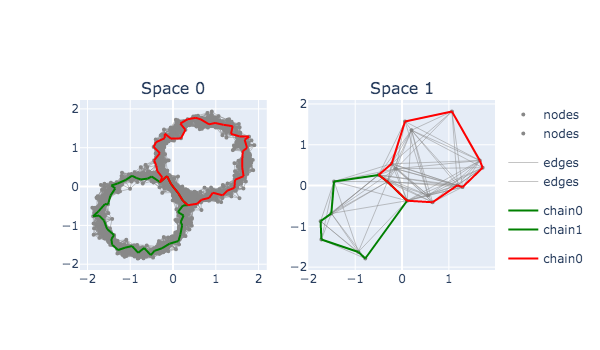}
    \includegraphics[width=0.49\linewidth]{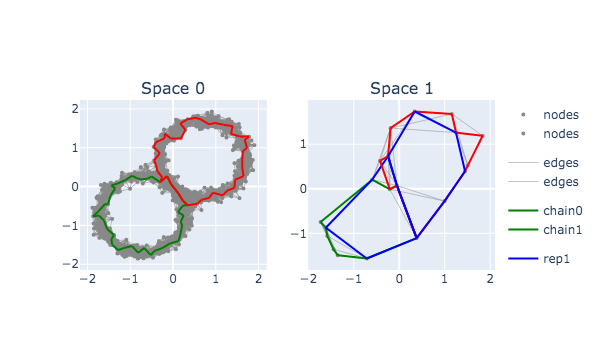}
    \includegraphics[width=0.49\linewidth]{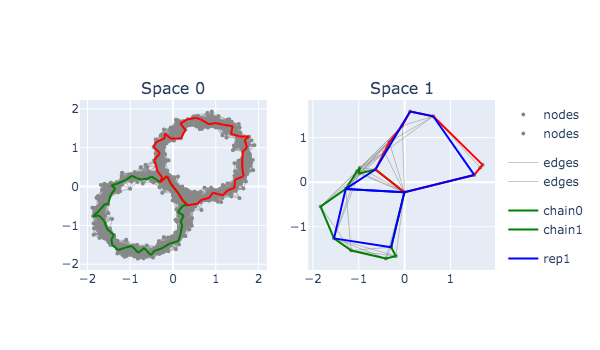}
    \includegraphics[width=0.49\linewidth]{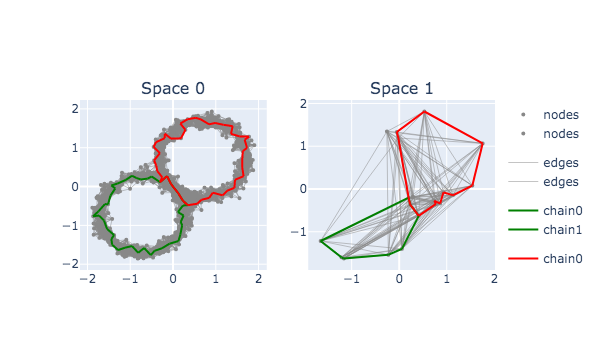}
    \includegraphics[width=0.49\linewidth]{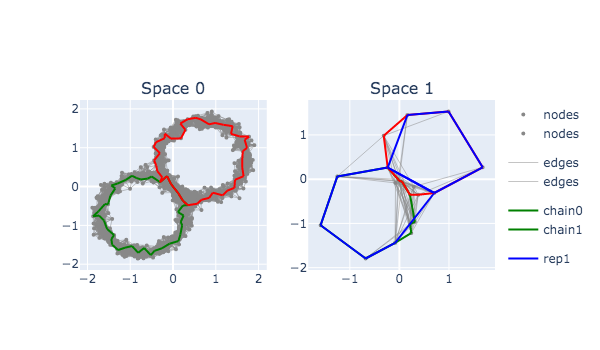}
    \includegraphics[width=0.49\linewidth]{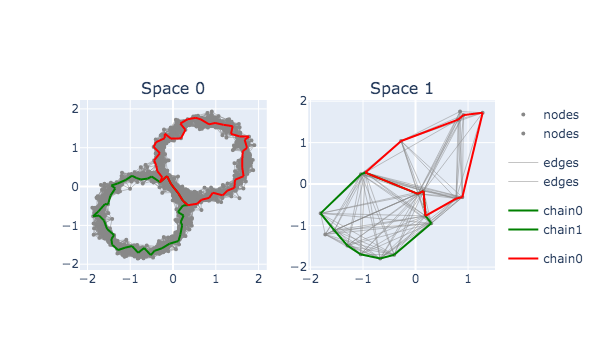}
    \caption{Projection maps of Figure-$8$ from full point cloud of size $1000$ to sub-samples of size $20$.}
    \label{fig:fig_8_20_pm}
\end{figure}

\begin{figure}
    \centering
    \includegraphics[width=0.49\linewidth]{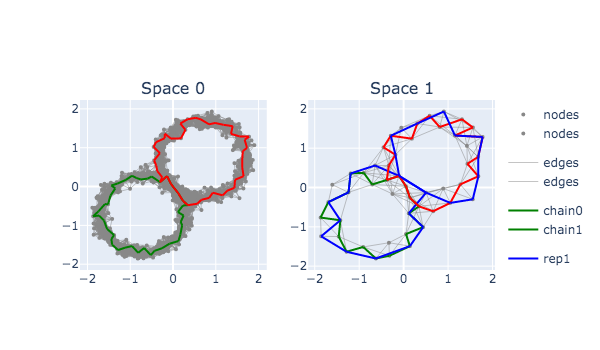}
    \includegraphics[width=0.49\linewidth]{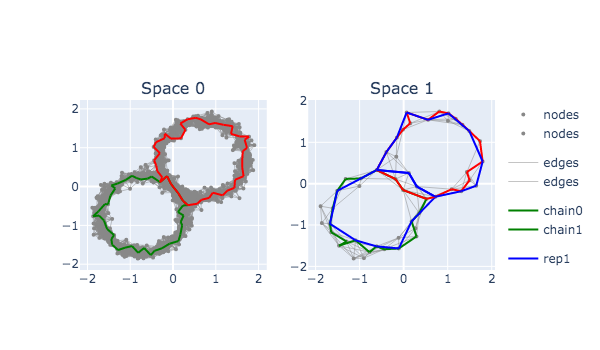}
    \includegraphics[width=0.49\linewidth]{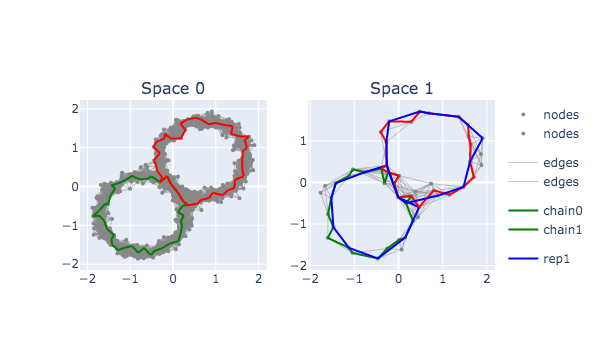}
    \includegraphics[width=0.49\linewidth]{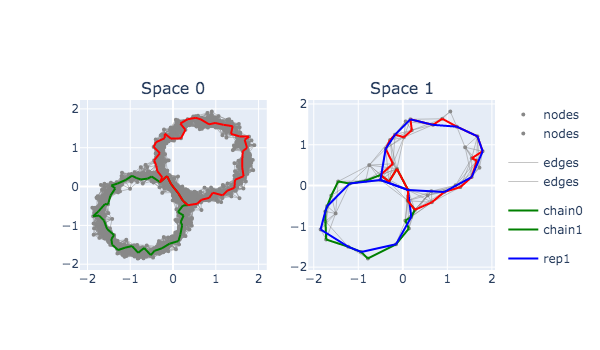}
    \includegraphics[width=0.49\linewidth]{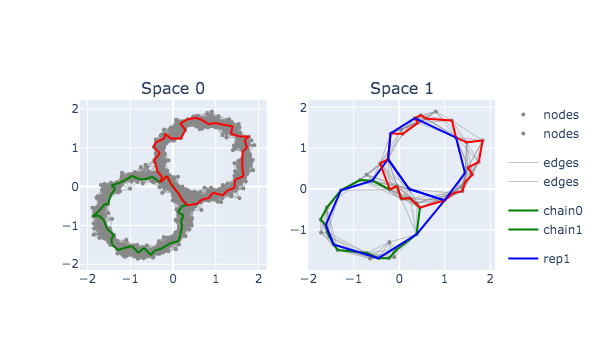}
    \includegraphics[width=0.49\linewidth]{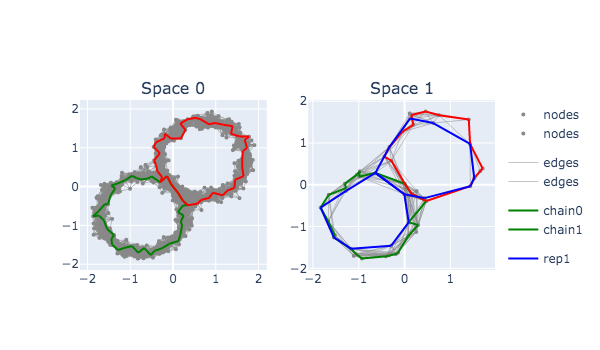}
    \includegraphics[width=0.49\linewidth]{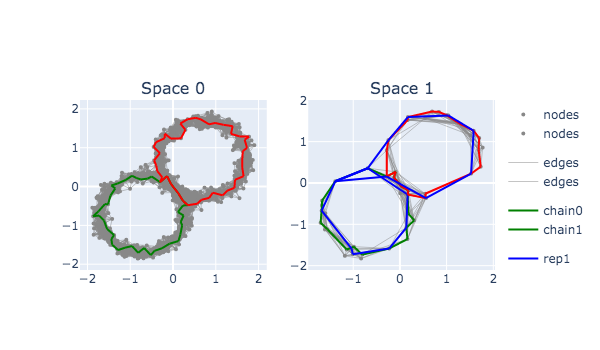}
    \includegraphics[width=0.49\linewidth]{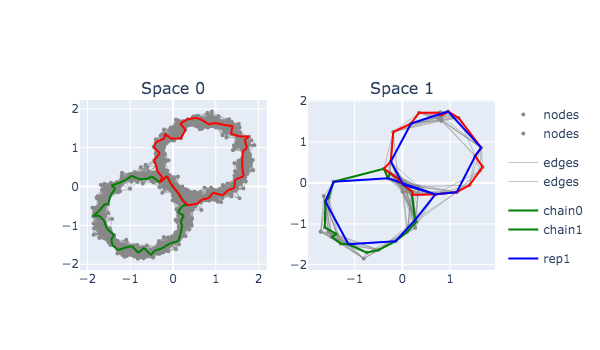}
    \includegraphics[width=0.49\linewidth]{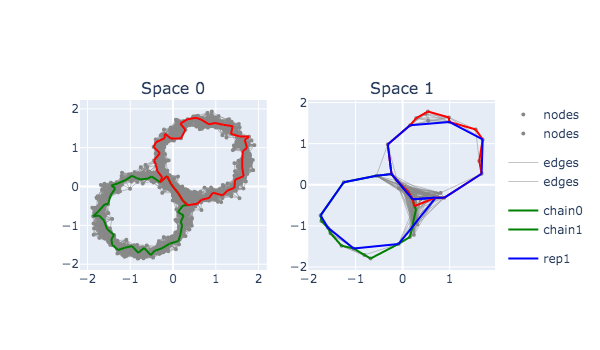}
    \includegraphics[width=0.49\linewidth]{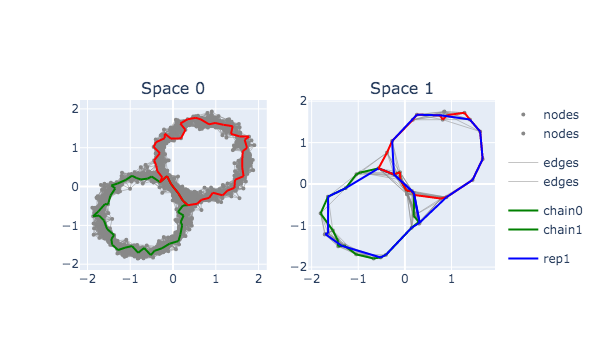}
    \caption{Projection maps of Figure-$8$ from full point cloud of size $1000$ to sub-samples of size $50$.}
    \label{fig:fig_8_50_pm}
\end{figure}

\begin{figure}
    \centering
    \includegraphics[width=0.49\linewidth]{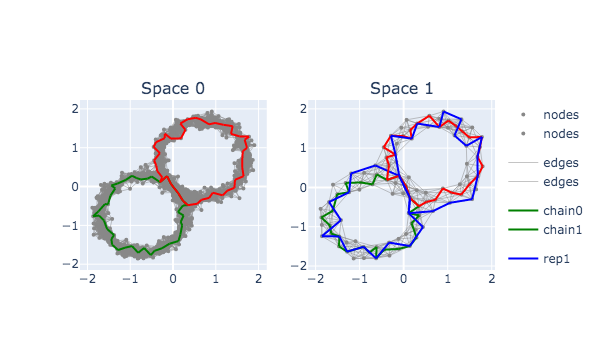}
    \includegraphics[width=0.49\linewidth]{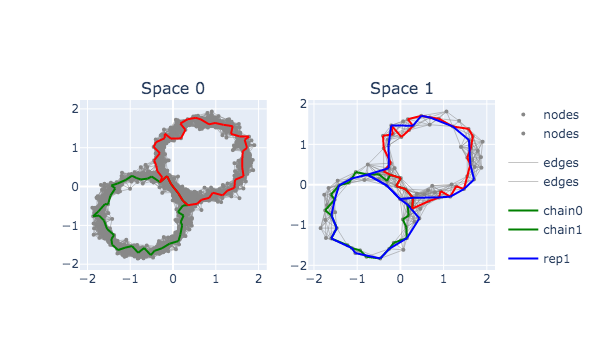}
    \includegraphics[width=0.49\linewidth]{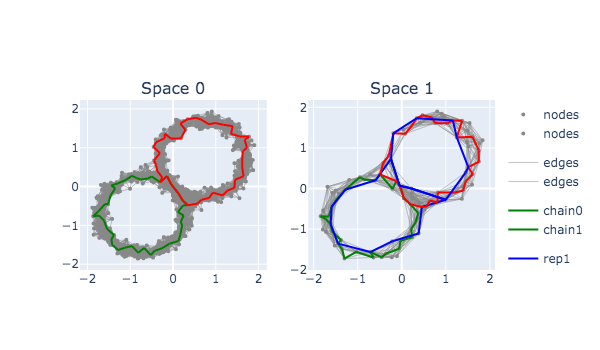}
    \includegraphics[width=0.49\linewidth]{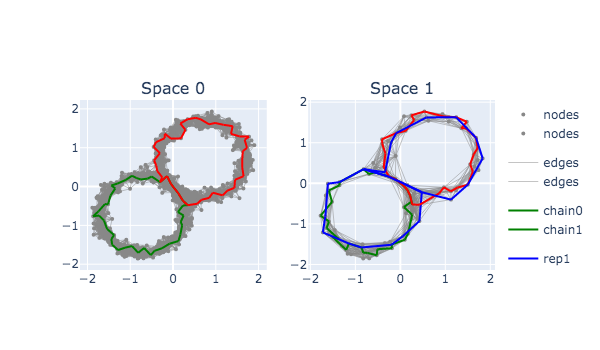}
    \includegraphics[width=0.49\linewidth]{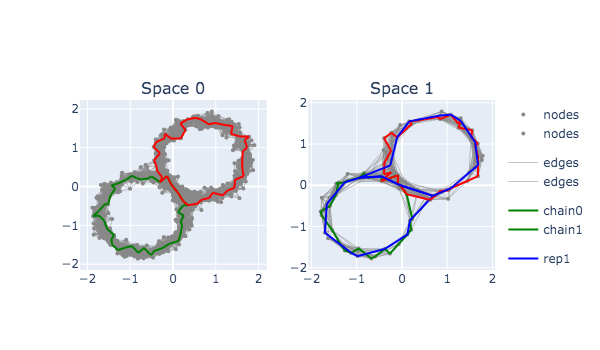}
    \includegraphics[width=0.49\linewidth]{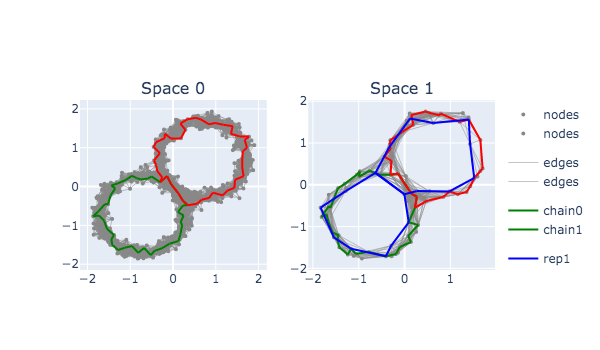}
    \includegraphics[width=0.49\linewidth]{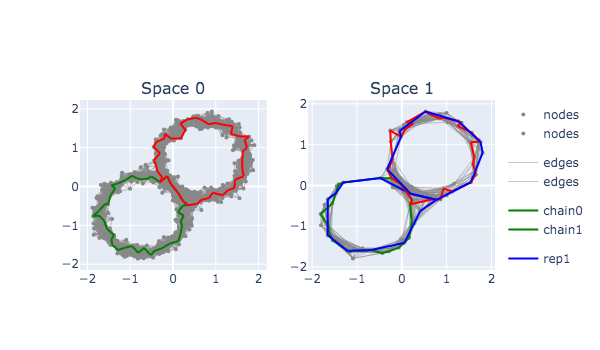}
    \includegraphics[width=0.49\linewidth]{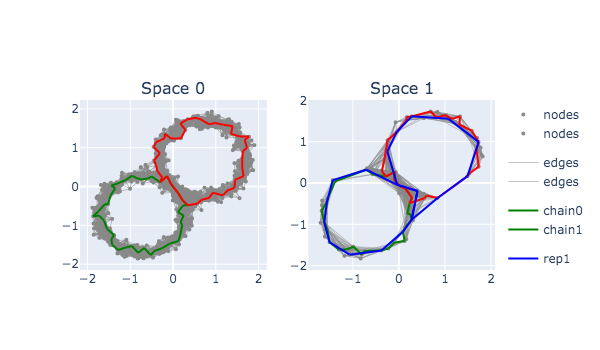}
    \includegraphics[width=0.49\linewidth]{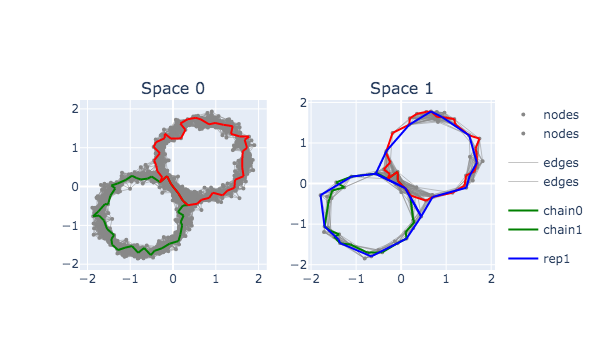}
    \includegraphics[width=0.49\linewidth]{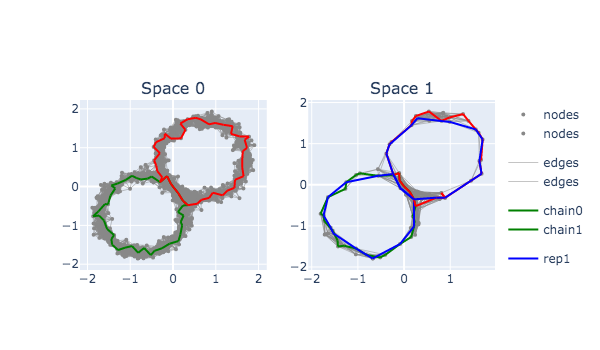}
    \caption{Projection maps of Figure-$8$ from full point cloud of size $1000$ to sub-samples of size $100$.}
    \label{fig:fig_8_100_pm}
\end{figure}

\begin{figure}
    \centering
    \includegraphics[width=0.49\linewidth]{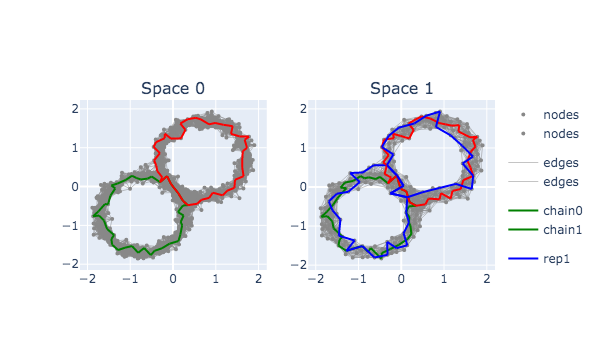}
    \includegraphics[width=0.49\linewidth]{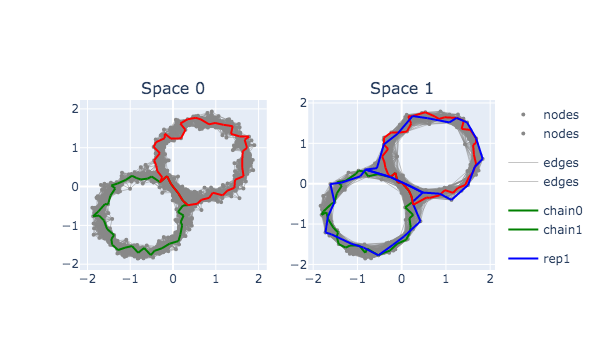}
    \includegraphics[width=0.49\linewidth]{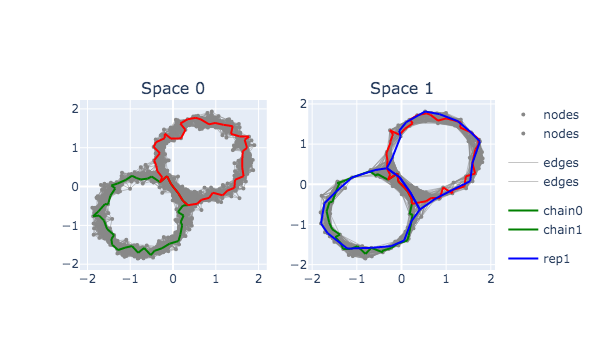}
    \includegraphics[width=0.49\linewidth]{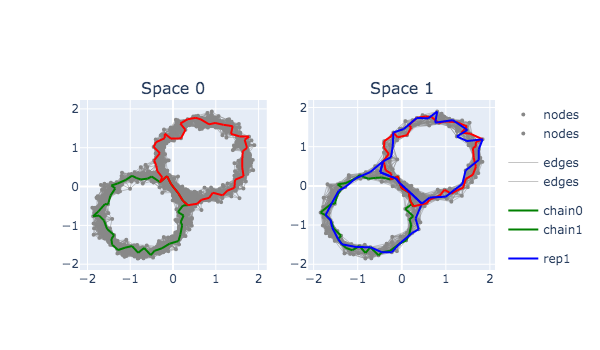}
    \includegraphics[width=0.49\linewidth]{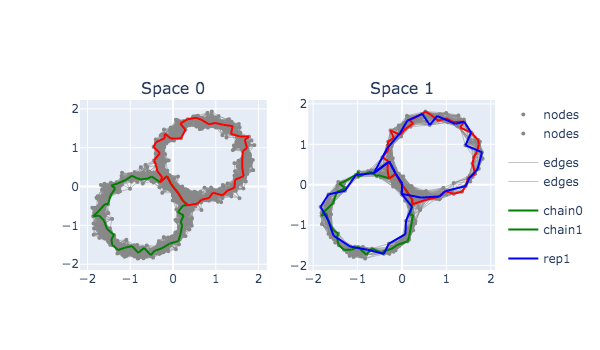}
    \includegraphics[width=0.49\linewidth]{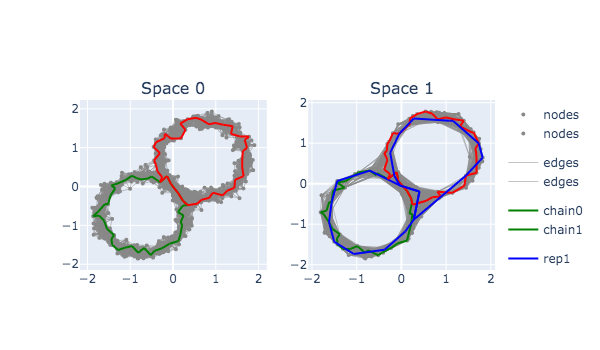}
    \includegraphics[width=0.49\linewidth]{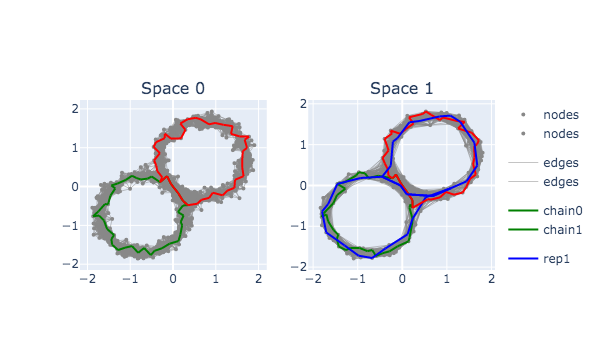}
    \includegraphics[width=0.49\linewidth]{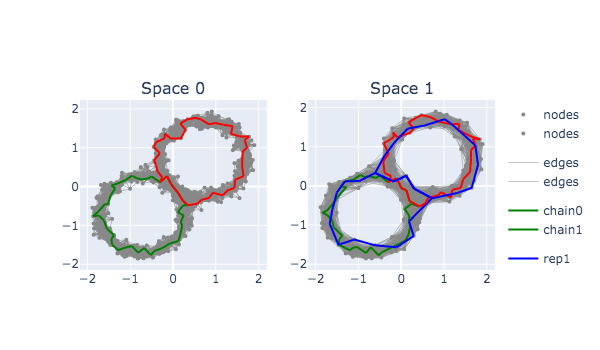}
    \includegraphics[width=0.49\linewidth]{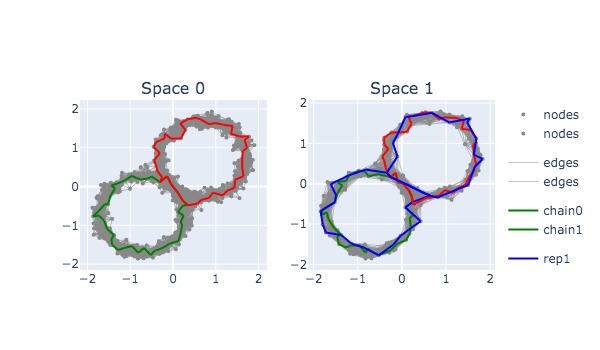}
    \includegraphics[width=0.49\linewidth]{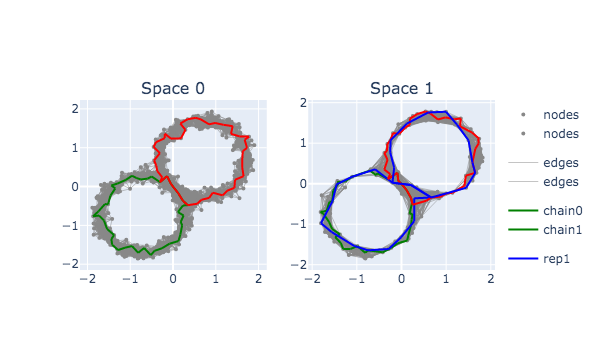}
    \caption{Projection maps of Figure-$8$ from full point cloud of size $1000$ to sub-samples of size $300$.}
    \label{fig:fig_8_300_pm}
\end{figure}
